# Supplementary material for: Concept-skill Transferability-based Data Selection for Large Vision-Language Models
Source: arXiv:2406.10995 source file (2024-10-02)
Supplement: Supplementary file 1 [file supplement_compare_to_tive.tex]

\begin{table*}[t]
    \tiny
    \vspace{-0.05in}
    \caption{\small We finetune LVLMs with coresets collected from the Vision-Flan~\citep{Xu2024visionflan} dataset with \textbf{16.7\% sampling ratio} for a single epoch. In the top table, we compare with baseline methods on multimodal evaluation benchmarks referring to~\citep{Xu2024visionflan}. At the bottom of the table, we show the results from the TIVE~\citep{Liu2024tive} where it finetunes the LVLMs for two epochs with the same 16.7\% selection ratio. SEED-I~\citep{seed_i} is a multiple-choice evaluation benchmark that estimates image understanding capabilities.}
    \vspace{-0.1in}
    \centering
    \resizebox{0.9\textwidth}{!}{

        \begin{tabular}{l c c c c c c c c a}
             \toprule
             {\textbf{Method}} & {\textbf{MMBench}} & {\textbf{MME}} & {\textbf{MM-Vet}} & {\textbf{POPE}} & {\textbf{SQA-I}} & {\textbf{SEED-I}} & {\textbf{Task}} & {\textbf{Gradient}} & {\textbf{\relp (\%)}}\\
             & {\textbf{en}} & & & & & & {\textbf{labels}} & {\textbf{Calculation}} & \\
             \midrule
             Full-Finetune &
             {\scriptsize 53.4} & {\scriptsize 1287.5} & {\scriptsize 25.6} & {\scriptsize 84.2} & {\scriptsize 61.3} & {\scriptsize - } & {\scriptsize $\times$ } & {\scriptsize $\times$ } & {\scriptsize 100}\\
             \cmidrule{0-9}
              Random &
             {\scriptsize 45.2} & {\scriptsize 1122.3} & {\scriptsize 26.1} & {\scriptsize 82.5} & {\scriptsize 60.9} & {\scriptsize - } & {\scriptsize $\times$ } & {\scriptsize $\times$ } & {\scriptsize 94.2}\\
                Self-Filter &
             {\scriptsize 28.6} & {\scriptsize 923.6} & {\scriptsize \textbf{30.0}} & {\scriptsize \textbf{83.3}} & {\scriptsize 59.3} & {\scriptsize - } & {\scriptsize $\times$ } & {\scriptsize \color{crimson}$\circ$ } & {\scriptsize 87.6}\\
                \cellcolor{gg}\ours (Ours) &
             \cellcolor{gg}{\scriptsize \textbf{56.7}} & \cellcolor{gg}{\scriptsize \textbf{1222.2}} & \cellcolor{gg}{\scriptsize 26.2} & \cellcolor{gg}{\scriptsize 81.9} & \cellcolor{gg}{\scriptsize \underline{63.8}} & \cellcolor{gg}{\scriptsize - } & \cellcolor{gg}{\scriptsize $\times$ } & \cellcolor{gg}{\scriptsize $\times$ } & \cellcolor{gg}{\scriptsize \textbf{101.0}}\\
             \midrule
             Full-Finetune & {\scriptsize - } & {\scriptsize - } & {\scriptsize - } & {\scriptsize 81.7} & {\scriptsize 65.6} & {\scriptsize 58.4} & {\scriptsize $\times$ } & {\scriptsize $\times$ } & {\scriptsize 100} \\
              \cmidrule{0-9}
             Random & {\scriptsize - } & {\scriptsize - } & {\scriptsize - } & {\scriptsize 81.1} & {\scriptsize 64.9} & {\scriptsize 56.8} & {\scriptsize $\times$ } & {\scriptsize $\times$ } & {\scriptsize 98.5} \\
             Length & {\scriptsize - } & {\scriptsize - } & {\scriptsize - } & {\scriptsize 81.8} & {\scriptsize 64.4} & {\scriptsize 56.8} & {\scriptsize $\times$ } & {\scriptsize $\times$ } & {\scriptsize 98.5} \\
             TIVE & {\scriptsize - } & {\scriptsize - } & {\scriptsize - } & {\scriptsize 81.5} & {\scriptsize 65.3} & {\scriptsize 57.4} & {\scriptsize \color{crimson}$\circ$ } & {\scriptsize \color{crimson}$\circ$ } & {\scriptsize 99.2} \\
             \bottomrule
        \end{tabular}
    }
    \label{tab:vision_flan_compare_to_tive}
    \vspace{-0.1in}
\end{table*}
