# Supplementary material for: Concept-skill Transferability-based Data Selection for Large Vision-Language Models
Source: arXiv:2406.10995 source file (2024-10-02)
Supplement: Supplementary file 2 [file supplement_curri_algo.tex]

\begin{figure*}[t]
\begin{minipage}{\textwidth}
    \centering
    \begin{algorithm}[H]
        \caption{\small \ours+ Curriculum Learning Algorithm}
        \label{alg:curri_algo}
        \begin{algorithmic}[1]
            \small
            \REQUIRE $K$: the number of clusters, $\gamma$: exploration rate, $\mu$: moving average rate, $T$: the number of rounds $S$: the number of steps per round, $\mathcal{D}=\{\mathcal{D}_1,\ldots,\mathcal{D}_K\}$: Dataset for $K$ clusters, $f_\theta$: training model
            \INIT $R_i=0$, $\mathcal{L}_{i,\text{past}}=0$\;\;$i\!\in\!\{1,2,\ldots,K\}$
            \FOR{$t = 1,2,\ldots,T$}
                \STATE $p_i(t)\!=\!(1-\gamma)\frac{R_i}{\sum_{j=1}^{K}}+\frac{\gamma}{K}$,\;\;$i\!\in\!\{1,2,\ldots,K\}$ \COMMENTARR{Calculate cluster selection distribution at step $t$}
                \FOR{$s = 1,2,\ldots,S$}
                    \STATE $D_i\sim p(t)$ \COMMENTARR{Select cluster $i$ from the step $t$ distribution}
                    \STATE $B\sim D_i$ \COMMENTARR{Sample batch from cluster $i$}
                    \STATE $R_i \leftarrow (1 - \mu)R_i + \mu (\mathcal{L}_{i,\text{past}} - \mathcal{L}(f_\theta,B))$ \COMMENTARR{Upate reward of cluster $i$}
                    \STATE $\mathcal{L}_{i,\text{past}}=\mathcal{L}(f_\theta,B)$
                    \STATE $\theta \leftarrow \theta - \eta\nabla_{\theta}\mathcal{L}(f_\theta,B)$ \COMMENTARR{Update model parameters}
                \ENDFOR
            \ENDFOR
        \end{algorithmic}
    \end{algorithm}
\end{minipage}
\vspace{-0.2in}
\end{figure*}
