# Supplementary material for: Concept-skill Transferability-based Data Selection for Large Vision-Language Models
Source: arXiv:2406.10995 source file (2024-10-02)
Supplement: Supplementary file 3 [file supplement_curriculum.tex]

\begin{table*}[t]
    \tiny
    \vspace{-0.1in}
    \caption{\small We perform a comparison with the curriculum learning baseline on various multimodal evaluation benchmarks. We finetune LVLMs with LLaVA-1.5~\citep{Liu2023llava15} dataset utilizing 20\% of the total steps for training. The best and the second best results are in \textbf{bold} and \underline{underlined}, respectively.}
    \vspace{-0.1in}
    \centering
    \resizebox{0.95\textwidth}{!}{

        \begin{tabular}{l c c c c c c c cc c a}
             \toprule
             {\textbf{Method}} & {\textbf{VQAv2}} & {\textbf{GQA}} & {\textbf{VizWiz}} & {\textbf{SQA-I}} & {\textbf{TextVQA}} & {\textbf{POPE}} & {\textbf{MME}} & \multicolumn{2}{c}{\textbf{MMBench}} & {\textbf{LLaVA-}} & {\textbf{\relp (\%)}}\\
             & & & & & & & & {\textbf{en}} & {\textbf{cn}} & {\textbf{Bench}} & \\
             \midrule
             Full-Finetune &
             {\scriptsize 79.1} & {\scriptsize 63.0} & {\scriptsize 47.8} & {\scriptsize 68.4} & {\scriptsize 58.2} & {\scriptsize 86.4} & {\scriptsize 1476.9} & {\scriptsize 66.1} & {\scriptsize 58.9} & {\scriptsize 67.9} & {\scriptsize 100}\\
             \cmidrule{0-11}
              Random &
             {\scriptsize \underline{75.7}} & {\scriptsize \textbf{58.9}} & {\scriptsize \underline{44.3}} & {\scriptsize 68.5} & {\scriptsize \underline{55.3}} & {\scriptsize 84.7} & {\scriptsize \textbf{1483.0}} & {\scriptsize 62.2} & {\scriptsize 54.8} & {\scriptsize 65.0} & {\scriptsize \underline{95.8}}\\
              Skill-it~\citep{Chen2023skillit} &
             {\scriptsize 75.4} & {\scriptsize \underline{56.9}} & {\scriptsize 42.4} & {\scriptsize \underline{69.7}} & {\scriptsize \textbf{56.0}} & {\scriptsize \underline{84.9}} & {\scriptsize 1370.5} & {\scriptsize \underline{62.9}} & {\scriptsize \underline{55.2}} & {\scriptsize \textbf{68.2}} & {\scriptsize 95.3}\\
              COINCIDE+ (Ours) &
             {\scriptsize \textbf{75.8}} & {\scriptsize \underline{56.9}} & {\scriptsize \textbf{49.3}} & {\scriptsize \textbf{69.9}} & {\scriptsize 53.9} & {\scriptsize \textbf{86.0}} & {\scriptsize \underline{1470.0}} & {\scriptsize \textbf{64.0}} & {\scriptsize \textbf{56.4}} & {\scriptsize \underline{67.6}} & {\scriptsize \textbf{97.5}}\\
             \bottomrule
        \end{tabular}
    }
    \label{tab:curriculum}
    \vspace{-0.2in}
\end{table*}
