# Supplementary material for: Concept-skill Transferability-based Data Selection for Large Vision-Language Models
Source: arXiv:2406.10995 source file (2024-10-02)
Supplement: Supplementary file 4 [file supplement_effect_hyperparameter.tex]

\begin{table}[t]
    \centering
    \tiny
    \caption{\textbf{Effect of hyperparameters.}}
    \vspace{-0.05in}
    \resizebox{0.65\linewidth}{!}{

    \begin{tabular}{c c c}
         \toprule
         {$\bm{K}$} & {$\bm{\tau}$} & {\textbf{\relp (\%)}}\\
         \midrule
         7500 & 0.1 & {96.2}\\
         \textbf{10000} & \textbf{0.1} & \textbf{97.4}\\
         12500 & 0.1 & {97.1}\\
         10000 & 0.05 & {96.1}\\
         10000 & 0.2 & {96.8}\\
         \bottomrule
    \end{tabular}
}
\label{tab:effect_hyperparameter}
\end{table}
