# Supplementary material for: Concept-skill Transferability-based Data Selection for Large Vision-Language Models
Source: arXiv:2406.10995 source file (2024-10-02)
Supplement: Supplementary file 5 [file supplement_neuron_activation.tex]

\begin{table}[t]
    \centering
    \tiny
    \caption{\small \textbf{Choice of multimodal neuron activation.}}
    \vspace{-0.05in}
    \resizebox{0.65\linewidth}{!}{

    \begin{tabular}{l c}
         \toprule
         {\textbf{Neuron Activation}} & \relp (\%)\\
         \midrule
         Boolean & 95.7\\
         Last layer & 96.5\\
         Intermediate layers (Ours) & \textbf{97.4}\\
         \bottomrule
    \end{tabular}
}
\label{tab:neuron_activation}
\end{table}
